# Supplementary material for: Improving External Communication of Automated Vehicles Using Bayesian Optimization
Source: arXiv:2501.10792 source file (2025-01-18)
Supplement: Supplementary file 1 [file additionals.tex]

\begin{comment}
    
\begin{table}[ht!]
\centering
\small
\caption{Results of Bayesian Analysis for Each Design Parameter including the Means and SD}
\begin{tabular}{lllll}
\hline
\textbf{Design Parameter} & \textbf{BF (± \%)} & \textbf{Female M (SD)} & \textbf{Male M (SD)} & \textbf{Evidence} \\
\hline
{Alpha} & 0.71 ± 0.02\% & 0.82 (0.15) & 0.86 (0.13) & inconclusive evid. for equality \\
\textit{Blue} & \textit{0.17 ± 0.05\%} & \textit{0.81 (0.12)} & \textit{0.81 (0.12)} &  \textit{moderate evid. for equality} \\
{Green} & {0.39 ± 0.03\%} & {0.80 (0.12)} & {0.83 (0.11)} &  inconclusive evid. for equality \\
{Red} & {1.40 ± 0.01\%} & {0.76 (0.16)} & {0.81 (0.17)} & inconclusive evid. for difference \\ \hdashline
\textit{Blink frequency} & \textit{0.19 ± 0.05\%} & \textit{0.79 (0.17)} & \textit{0.80 (0.17)} & \textit{moderate evid. for equality} \\
\textit{Horizontal width} & \textit{0.22 ± 0.05\%} & \textit{0.83 (0.14)} & \textit{0.85 (0.13)} & \textit{moderate evid. for equality} \\
\textit{Vertical position} & \textit{0.19 ± 0.05\%} & \textit{0.76 (0.16)} & \textit{0.75 (0.15)} & \textit{moderate evid. for equality} \\
{Vertical width} & 0.37 ± 0.03\% & 0.79 (0.15) & 0.82 (0.15) & inconclusive evid. for equality \\ \hdashline
\textit{Volume} & \textit{0.21 ± 0.05\%} & \textit{0.84 (0.13)} & \textit{0.82 (0.13)} & \textit{moderate evid. for equality} \\
\hline
\end{tabular}
\label{tab:bf_parameters}
\end{table}
\end{comment}
